# Supplementary material for: Modelling the influence of photospheric turbulence on solar flare statistics
Source: arXiv:1410.4542 source file (2014-10-16)
Supplement: Supplementary file 1 [file supp_information.pdf]

## SUPPLEMENTARY FIGURES

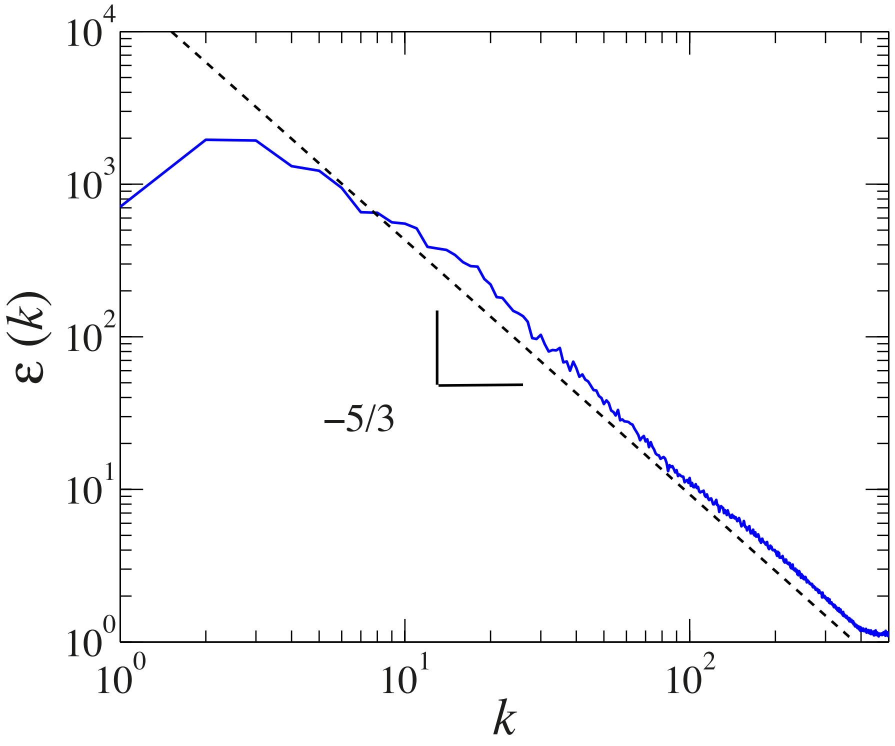


**Supplementary Figure** 1. **Energy spectrum of the photospheric turbulence flow.** For different system sizes $L$, the fluid first evolves without the magnetic flux tubes until it reaches the turbulent regime. Here, we can observe the energy spectrum, $\epsilon(k)$, for the largest system size of $L = 2048$, before the magnetic flux tubes are inserted. The power-law distribution extends for two decades showing that the fluid is in the turbulent regime. The dashed line denotes the Kolmogorov exponent.

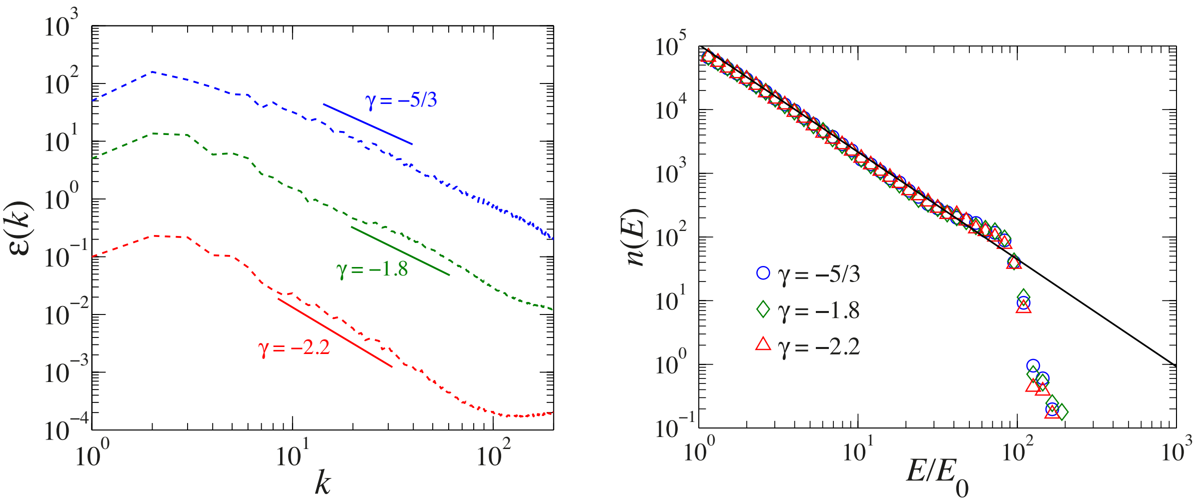


**Supplementary Figure** 2. **Induced energy spectrum of the photospheric turbulence flow.** In the left panel, we show the energy spectrum, $\epsilon(k)$, of the photospheric turbulent flow, using three different induced exponents within the range of experimental observations. In the right panel, we observe the distribution of flare energies evaluated with our numerical model for different values of the induced exponent $\gamma$. For this purpose, we have set $\mu = 2.4$, and 2.8, to obtain $\gamma = -1.8$, and $-2.2$, respectively. We have considered only the case of interacting loops ($\lambda_{\mathrm{R}} < 1$), with a system size $L = 512$, aspect ratio $r_{\mathrm{c}}/R = 0.1$ and number of magnetic flux tubes $N = 400$. We find that the power law remains unchanged suggesting that our results do not depend on the exponent chosen for the energy spectrum of the turbulent flow, at least within the range of experimental observations.

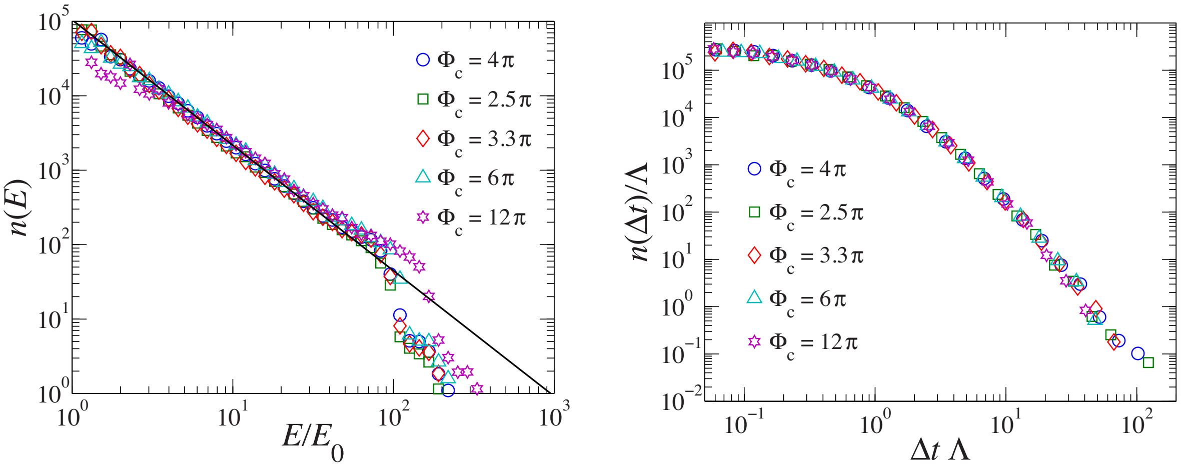


**Supplementary Figure 3. Universal behavior of the Solar flare energies and temporal organization by changing the critical twist $\Phi_c$.** In the left panel, we observe the distribution of flare energies evaluated with our numerical model for different values of the critical twist $\Phi_c$, reported in the literature from theoretical, numerical, and experimental observations [1–3]. We have considered only the case of interacting loops ($\lambda_R < 1$), with a system size $L = 512$, aspect ratio $r_c/R = 0.1$ and number of magnetic flux tubes $N = 400$. Within the range of experimental observations and theoretical predictions we find that the power law remains unchanged showing that our results do not depend on the value chosen for the critical twist of the kink instability. In the right panel, the waiting time distribution for solar flares is shown for different critical twist values. Here we can observe as well that the complex temporal organization is invariant under changing $\Phi_c$.

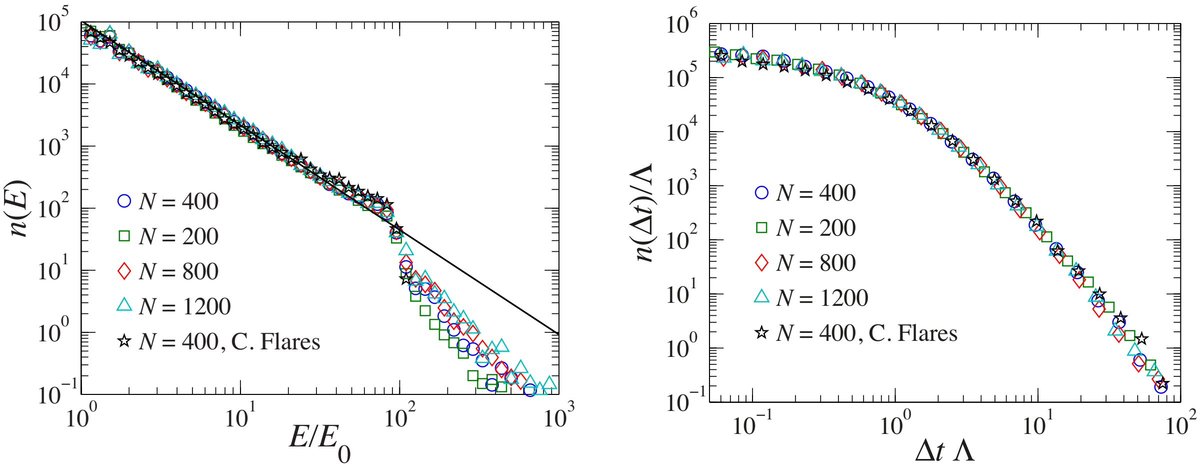


**Supplementary Figure** 4. **Universal behavior of the Solar flare energies and temporal organization by changing the number of magnetic flux tubes** $N$**.** In the left panel, we observe the distribution of flare energies evaluated with our numerical model for different number of inserted magnetic flux tubes $N$. We have considered only the case of interacting loops ($\lambda_R < 1$), with a system size of $L = 512$, aspect ratio of $r_c/R = 0.1$, and critical twist $\Phi_c = 4\pi$. We find that the power law remains unchanged showing that our results do not depend on the number of magnetic flux tubes. In our model, if two or more flare events occur at the same time we sum their energies and count them as a single event. However, one can consider the case where these events are treated as independent ones and use fractional time steps for the temporal organization (they are located within a single time step and separated by equal intervals with random order). We have also included this case (denoted by C. Flares, from concurrence flares) using $N = 400$, where we see that once again the power-law distribution remains unchanged. In the right panel, the waiting time distribution for solar flares for the same cases than for the left panel are presented. Here we can observe as well that the complex temporal organisation is invariant for different tube densities.

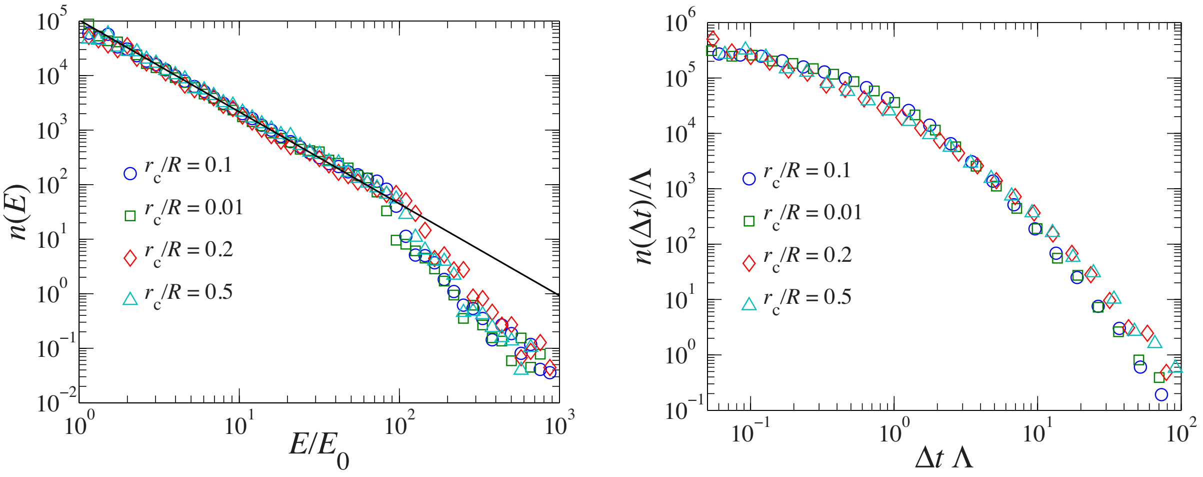


**Supplementary Figure** 5. **Universal behaviour of the Solar flare energies and temporal organisation by changing the magnetic flux tube aspect ratio** $r_{\rm c}/R$**.** In the left panel, we observe the distribution of flares evaluated with our numerical model for different values of the aspect ratio $r_{\rm c}/R$. We have considered only the case of interacting loops ($\lambda_{\rm R} < 1$), for a system size $L = 512$, critical twist of $\Phi_{\rm c} = 4\pi$, and number of magnetic flux tubes $N = 400$. We find that the power law remains unchanged showing that our results do not depend on the value chosen for the aspect ratio of the magnetic flux tubes. In the right panel, the waiting time distribution for solar flares is shown for the same cases than for the left panel. Here we can observe as well that the complex temporal organisation is invariant under changing $r_{\rm c}/R$. Notice that by increasing $r_{\rm c}/R$, the lower energy cutoff $E_0$ also needs to be increased, since the minimum flare energy gets larger, therefore, for $r_{\rm c}/R = 0.01$, 0.1, and 0.2, we set $E_0 = 10$, whereas for $r_{\rm c}/R = 0.5$ we set $E_0 = 10^3$.

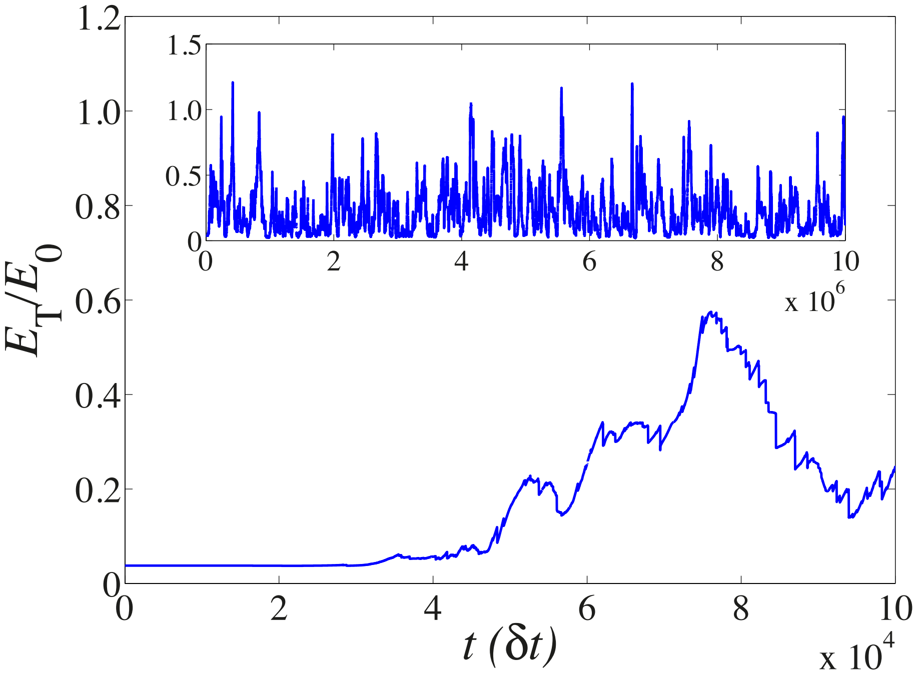


**Supplementary Figure** 6. **Total magnetic energy stored by the system as a function of time.** The total magnetic energy of the system is computed by summing up the energy of all magnetic flux tubes. Main panel: we can observe that the total energy increases due to the turbulence flow, and then, suddenly decreases due to the energy released by flares. Inset: In a larger interval of time, we see that the processes of magnetic flux tube reconnection and injection of energy by the turbulent flow coexist producing valleys and peaks in the total energy of the system. We have set $E_0 = 10^4$, and considered only the case of interacting loops with relaxation ($\lambda_{\mathrm{R}} < 1$), with a system size of $L = 512$, aspect ratio of $r_{\mathrm{c}}/R = 0.1$, critical twist $\Phi_{\mathrm{c}} = 4\pi$, and $N = 100$.

## SUPPLEMENTARY TABLES

| $L$ | $Re$ | $N$ | $N_{\rm e}$ |
|---|---|---|---|
| 128 | $9 \times 10^3$ | 100 | 200000 |
| 256 | $1.7 \times 10^4$ | 200 | 200000 |
| 512 | $3.5 \times 10^4$ | 400 | 200000 |
| 1024 | $6.0 \times 10^4$ | 800 | 175100 |
| 2048 | $1.1 \times 10^5$ | 1600 | 150000 |

**Supplementary Table** I. **Numerical details on the magnetic flux tubes and fluid simulations.** For every system size $L$, we measure the Reynolds number $Re = u_{\rm rms}L/\nu$, using as characteristic velocity the root-mean-square (rms) of the velocity field, more precisely $u_{\rm rms} = \langle|\mathbf{u}|\rangle$, where $\langle ... \rangle$ denotes the spatial average in the simulated region, and the kinematic viscosity of the fluid $\nu = 10^{-3}$. In this Supplementary Table we also find the number of loops $N$ inserted for each case and the number of recorded solar flare events $N_{\rm e}$.

## SUPPLEMENTARY REFERENCES

[1] Hood, A. W. & Priest, E. R. Kink instability of solar coronal loops as the cause of solar flares. *Sol. Phys.* **64**, 303–321 (1979).

[2] Srivastava, A. K., Zaqarashvili, T. V., Kumar, P. & Khodachenko, M. L. Observation of kink instability during small b5.0 solar flare on 2007 june 4. *The Astrophysical Journal* **715**, 292 (2010).

[3] Török, T. & Kliem, B. Confined and ejective eruptions of kink-unstable flux ropes. *The Astrophysical Journal Letters* **630**, L97 (2005).
